# Supplementary material for: Physics-based Differentiable Depth Sensor Simulation
Source: arXiv:2103.16563 source file (2021-08-06)
Supplement: Supplementary file 1 [file 5_supmat.tex]

\vspace{2em}

\appendix
\beginsupplement

\noindent
\pdfbookmark[0]{Supplementary Material}{sup_mat}
{\Large\textbf{Supplementary Material} \vspace{1em}}

\subsection{Implementation}
\bp{todo}

\subsection{Additional Results}
\bp{todo}

Table~\ref{tab:supmat_linemod} presents a detailed picture of the various solutions commonly used to trained visual recognition applications in scarce-data setups (basic or simulation-based synthetic image generation, static or GAN-based online image augmentations, \etc) and their performance on the task at hand. The various schemes are further sorted \wrt multiple parameters. For their respective image rendering phases, we consider (a) the chosen rendering solution, (b) the addition or not of realistic clutter in the 3D scene (\ie, populating the scene with a ground surface and other 3D objects around the target one), (c) and the optional post-processing applied to rendered images before their persistence (\eg, applying statistical noise or passing the images through a pre-trained GAN). During each training iteration of $T$, we also consider if and how the synthetic training images are augmented (\eg, through manually-parameterized random 2D operations or a trained-along generative network). As such, Table~\ref{tab:linemod} also reads as an ablation study of domain adaptation and simulation methods, ours included.

Analyzing the results, we can first observe the correlation between classification and pose estimation results, and their wide performance range. Network instances trained on non-cluttered, non-augmented synthetic images completely fail the task. Corroborating the observations made by other researchers \wrt synthetic RGB data~\cite{hodavn2019photorealistic,denninger2019blenderproc}, the simple step of adding some pseudo-realistic clutter to the 3D scenes before rendering greatly improves the relevance of synthetic images. Moreover, regardless of the quality of rendered images, the addition of online augmentations (\eg, random distortion, depth jittering, \etc) consistently provides an accuracy boost by virtually increasing the training set size and variability \cf domain randomization theory~\cite{domainrandom}. Interestingly, unsupervised adversarial domain adaptation methods (\textit{PixelDA}~\cite{bousmalis2017unsupervised}, \textit{DRIT++}~\cite{lee2020drit++}, \textit{DeceptionNet}~\cite{zakharov2019deceptionnet}) perform significantly better than previous depth simulation tools (\textit{BlenSor}~\cite{gschwandtner2011blensor}, \textit{DepthSynth}~\cite{planche2017depthsynth}), further giving credits to the domain randomization approach. However, it is primordial to note that simulation-based tools have superior generalization capability. While the CNN-based domain adaptation methods perform well on images of known objects, they cannot generalize to new classes without having to be retrained, and most require real images for that. 

\begin{table*}[t]
\centering
\caption{\textbf{Comparative and ablative study}, measuring the impact of domain adaptation, domain randomization, and sensor simulation techniques applied to synthetic training images during the training of a CNN~\cite{ganin2015} for depth-based instance classification and pose estimation on the \textit{Cropped LineMOD} dataset~\cite{wolhlart2012}.
Results highlight the benefits of trainable ray-tracing-based sensor simulation and post-processing, and of augmenting the 3D scenes and 2D images with random clutter and transforms.}
\label{tab:supmat_linemod} 
\resizebox{1\linewidth}{!}{
% \label{tab:gan_comp}
\begin{tabu}{@{}cc|ccc|c|ccc|c@{\hskip 10pt}c@{}}
\toprule
\multicolumn{2}{c}{\multirow{2}{*}{\shortstack{\textbf{Training Data}\\\textbf{Source}}}} & 
\multicolumn{3}{|c|}{\textbf{3D Rendering}} & 
\multicolumn{1}{|c|}{\multirow{2}{*}{\shortstack{\textbf{Online}\\\textbf{2D Aug.}}}} & \multicolumn{3}{|c|}{\textbf{Training Req.}} &  
\multirow{2}{*}{\shortstack{\textbf{Classification}\\\textbf{Accuracy}$^\nearrow$}} &
\multirow{2}{*}{\shortstack{\textbf{Rotational}\\\textbf{Error}$^\searrow$}}
\\
\cmidrule(lr){3-5}\cmidrule(lr){7-9}
& & ray-tracing & clutter & post-proc. & & $|\theta_G|$ & $|\theta_D|$ & $X^r_{trn}$ \\

\midrule

\multicolumn{2}{c|}{\multirow{2}{*}{Basic}} &
&   &	  &	 					 &	 					& 			 &				  &		21.3\% &	91.8$^{\circ}$	
\\
&	&	&   $\checkmark$ & &	 					 &	 					& 			 &				  &		55.8\% &	61.0$^{\circ}$
\\
&   &	  &	 					& &	img-op			&	& 			 &				  &		42.8\% &	67.3$^{\circ}$
\\
&	&   &	 $\checkmark$ &	 					 &	img-op				& & 			 &				  &		74.7\% &	49.1$^{\circ}$
\\
\cmidrule(lr){1-11}

\parbox[t]{2mm}{\multirow{8}{*}{\rotatebox[origin=c]{90}{Domain Adaptation}}} &
\multirow{2}{*}{\textit{PixelDA}} &
  &	  &	 					 &	GAN					& 	1.96M	 &	693k &		 $\checkmark$ &		65.8\% &	56.5$^{\circ}$	
\\
&&   &	 $\checkmark$ &	 					 &	GAN					& 	1.96M	 &	693k &		 $\checkmark$ &		85.7\% &	40.5$^{\circ}$	
\\
\cmidrule(lr){2-11}

& 
\multirow{4}{*}{\textit{DRIT++}} 
&   &	  &	GAN					 &	 					& 	21.3M &	33.1M &	 $\checkmark$ &		36.2\% &	91.9$^{\circ}$	\\
& &   &	  &	GAN					 &	img-op				& 	21.3M &	33.1M &	 $\checkmark$ &		62.5\% &	89.1$^{\circ}$	\\
& &   &	 $\checkmark$ &	GAN					 &	 					& 	21.3M &	33.1M &	 $\checkmark$ &		68.0\% &	60.8$^{\circ}$	\\
& &   &	 $\checkmark$ &	GAN					 &	img-op				& 	21.3M &	33.1M &	 $\checkmark$ &		87.7\% &	39.8$^{\circ}$	\\
\cmidrule(lr){2-11}

&
\multirow{2}{*}{\textit{DeceptionNet}}
&   &	  &	 					 &	UNet + diff img-op	& 	1.54M	 &			 &	  &		37.3\% &	59.8$^{\circ}$	\\
&&   &	 $\checkmark$ &	 					 &	UNet + diff img-op	& 	1.54M	 &			 &	  &		89.2\% &	50.1$^{\circ}$	\\
\cmidrule(lr){1-11}

\parbox[t]{2mm}{\multirow{12}{*}{\rotatebox[origin=c]{90}{Sensor Simulation}}}  &
\multirow{4}{*}{\textit{DepthSynth}}
&  $\checkmark$ &	  &	stat. noise			 &	 					& 			 &			 &	  &		17.1\% &	87.5$^{\circ}$	\\
&&  $\checkmark$ &	  &	stat. noise			 &	img-op				& 			 &			 &	  &		45.6\% &	65.4$^{\circ}$	\\
&&  $\checkmark$ &	 $\checkmark$ &	stat. noise			 &	 					& 			 &			 &	  &		71.5\% &	52.1$^{\circ}$	\\
&&  $\checkmark$ &	 $\checkmark$ &	stat. noise			 &	img-op				& 			 &			 &	  &		76.6\% &	45.4$^{\circ}$	\\
\cmidrule(lr){2-11}

&
\multirow{4}{*}{\textit{BlenSor}}
&  $\checkmark$ &	  &	stat. noise			 &	 					& 			 &			 &	  &		14.9\% &	90.1$^{\circ}$	\\
&&  $\checkmark$ &	  &	stat. noise			 &	img-op				& 			 &			 &	  &		47.8\% &	61.0$^{\circ}$	\\
&&  $\checkmark$ &	 $\checkmark$ &	stat. noise			 &	 					& 			 &			 &	  &		67.5\% &	63.4$^{\circ}$	\\
&&  $\checkmark$ &	 $\checkmark$ &	stat. noise			 &	img-op				& 			 &			 &	  &		82.6\% &	41.4$^{\circ}$	\\
\cmidrule(lr){2-11}

&
\multirow{4}{*}{\shortstack{\textit{DDS}\\(untrained)}} 
&  $\checkmark$ &	  &	 					 &	 					& 			 &			 &	  &		15.6\% &	91.6$^{\circ}$	\\
&&  $\checkmark$ &	  &	 					 &	img-op				& 			 &			 &	  &		50.0\% &	68.9$^{\circ}$	\\
&&  $\checkmark$ &	 $\checkmark$ &	 					 &	 					& 			 &			 &	  &		69.7\% &	67.6$^{\circ}$	\\
&&  $\checkmark$ &	 $\checkmark$ &	 					 &	img-op				& 			 &			 &	  &		89.6\% &	39.7$^{\circ}$	\\
\cmidrule(lr){1-11}

\parbox[t]{2mm}{\multirow{7}{*}{\rotatebox[origin=c]{90}{Combined}}} &
\multirow{6}{*}{\textit{DDS}}
&  $\checkmark$ &	  &	stat. noise			 &	 					& 	4		 &	693k	 &	 $\checkmark$ &		21.3\% &	80.9$^{\circ}$	\\
&&  $\checkmark$ &	  &	stat. noise			 &	img-op				& 	4		 &	693k	 &	 $\checkmark$ &		51.6\% &	63.3$^{\circ}$	\\
&&  $\checkmark$ &	 $\checkmark$ &	stat. noise			 &	 					& 	4		 &	693k	 &	 $\checkmark$ &		81.2\% &	49.1$^{\circ}$	\\
&&  $\checkmark$ &	 $\checkmark$ &	stat. noise			 &	img-op				& 	4		 &	693k	 &	 $\checkmark$ &		90.5\% &	39.4$^{\circ}$	\\
&&  $\checkmark$ &	 $\checkmark$ &	stat. noise, conv x2 &	 					& 	2535	 &	693k	 &	 $\checkmark$ &		85.5\% &	45.4$^{\circ}$	\\
&&  $\checkmark$ &	 $\checkmark$ &	stat. noise, conv x2 &	img-op				& 	2535	 &	693k	 &	 $\checkmark$ &		93.0\% &	31.3$^{\circ}$	\\

\cmidrule(lr){2-11}
&
\multicolumn{1}{c|}{Real Imgs + \textit{DDS}}
&  $\checkmark$ &	 $\checkmark$ &	stat. noise, conv x2 &	img-op				& 	2535	 &	693k	 &	 $\checkmark$ &		\textbf{97.8\%} &	\textbf{25.1$^{\circ}$}	\\
\cmidrule(lr){1-11}

\multicolumn{2}{c|}{Real Imgs} &
& & & & & &  & 95.4\% &	35.0$^{\circ}$\\

\bottomrule
\end{tabu}
}
%	\vspace{0.4cm}   
\end{table*}
